# Supplementary material for: Classical Analog Emulation of Quantum Circuits via Time-Averaged Dynamic States
Source: arXiv:2601.02977 source file (2026-10-24)
Supplement: Supplementary file 1 [file prapplied_supp.tex]

% Supplemental Material for:
% "Classical Analog Emulation of Quantum Circuits via Time-Averaged Dynamic States"
% PRX Quantum Submission

\documentclass[aps,prapplied,onecolumn,superscriptaddress,floatfix,amsmath,amssymb]{revtex4-2}

%%% PACKAGES
\usepackage{graphicx}
\graphicspath{{./figures/}}
\usepackage{dcolumn}
\usepackage{bm}
\usepackage{braket}
\usepackage{mathtools}
\usepackage{physics}
\usepackage{amsmath,amsthm,amssymb,amsfonts}
\usepackage{booktabs}
\usepackage{xr}
\externaldocument{prapplied_main}
\usepackage{hyperref}
\usepackage{comment}
\usepackage{tikz}
\usetikzlibrary{arrows.meta,decorations.pathreplacing,shapes.geometric,positioning,fit,calc}
\usepackage{pgfplots}
\pgfplotsset{compat=1.18}
\usepackage{xcolor}
\usepackage{subcaption}
\usepackage{circuitikz}
%\usetikzlibrary{circuits.ee.IEC}
% Left-align section and subsection titles
\usepackage{titlesec}
\titleformat{\section}{\large\bfseries}{\thesection.}{0.6em}{}
\titleformat{\subsection}{\normalsize\bfseries}{\thesubsection}{0.6em}{}
\titleformat{\subsubsection}{\normalsize\itshape}{\thesubsubsection}{0.6em}{}

%%% THEOREM ENVIRONMENTS (reusing labels from main)
\newtheorem{theorem}{Theorem}
\newtheorem{lemma}[theorem]{Lemma}

%%% MACROS

\newcommand{\avgT}[1]{\left\langle #1 \right\rangle_T}
\newcommand{\avginf}[1]{\left\langle #1 \right\rangle_\infty}
\newcommand{\innprod}[2]{\left\langle #1,\, #2\right\rangle}

\begin{document}

\begin{center}
\large\textbf{Supplemental Material}\\[0.3em]
\normalsize\textit{Classical Analog Emulation of Quantum Circuits
via Time-Averaged Dynamic States}
\end{center}
\vspace{1em}

% --------------------------------------------------------
\appendix
\setcounter{section}{0}
\renewcommand{\thesection}{S\arabic{section}}
\renewcommand{\theequation}{S\arabic{equation}}
\setcounter{equation}{0}

\section{Unraveled 2-qubit gates}
\label{sup:sec:unravel_gate_examples}
% ============================================================

The main text (Sec.~\ref{subsec:2qubit_gate}) establishes the general gate-unraveling construction: any $2$-qubit unitary $\hat{U}$ can be written as
\begin{equation}
    \hat{U} = \avgT{\hat{S}_1(t)\otimes\hat{S}_2(t)},
\end{equation}
where $\hat{S}_1(t)$ and $\hat{S}_2(t)$ are time-varying $2\times2$ matrices whose elements are drawn from a set of orthonormal signals $\{s_k(t)\}$.  The construction is general but abstract; this section works out explicit signal matrices for four concrete gates that appear in the main text or in the hardware prototype.  The CNOT gate (Sec.~\ref{sup:sec:unravel_gate_examples} below) exploits the block-diagonal structure of the gate to reduce the required signals from four to two; it is the gate implemented in the analog prototype (Sec.~\ref{sup:sec:S_hardware_design}).  The CZ gate achieves the same signal economy via a superposition on the target-qubit matrix.  The SWAP gate, which has non-zero off-diagonal blocks, genuinely requires four distinct orthonormal signals.  Finally, the $\hat{R}_Y\!\otimes\hat{I}$ example illustrates \emph{passive} layers: separable gates that require no oscillating signals and are implemented as static matrix multiplications, serving as building blocks for the layer decomposition described in the main text.
\subsection{CNOT gate}
This gate has four non-zero entries, so the general construction of $\hat{S}_1(t)$ and $\hat{S}_2(t)$ requires four signals. Exploiting its block-diagonal structure reduces this to two:
\begin{equation}
    \hat{\mathrm{CNOT}} = \avgT{\begin{pmatrix}s_1 & 0\\0 & s_2\end{pmatrix}
    \otimes\begin{pmatrix}s_1^* & s_2^*\\s_2^* & s_1^*\end{pmatrix}},
    \label{eq:CNOT_unravel_supp}
\end{equation}
where $s_1 = e^{\mathrm{i}\Omega t}$ and $s_2 = e^{\mathrm{i}2\Omega t}$ are two orthonormal harmonics of the single base frequency $\Omega$. The control qubit operator selects between identity and flip using the same pair of signals that drives the target qubit's flip operation.  Since the CNOT occupies a single active layer, only one BF $\Omega$ is required; the $\mathbb{Q}$-independence condition does not arise here (it becomes relevant only when multiple active layers each need a distinct BF).  %This structure directly reproduces the phase kickback effect: for input $\ket{+}\otimes\ket{-}$, the emulated CNOT outputs $\ket{-}\otimes\ket{-}$ (verified experimentally, Sec.~\ref{subsec:experimental_results}).

\subsection{CZ gate}
The controlled-$Z$ gate $\hat{CZ} = \mathrm{diag}(1,1,1,-1)$ differs from CNOT only in that the target qubit acquires a phase rather than a bit flip when the control is $\ket{1}$.  Its unraveling uses the same two signals $s_1,s_2$ with a superposition on the target qubit:
\begin{equation}
    \hat{CZ} = \avgT{\begin{pmatrix}s_1 & 0\\0 & s_2\end{pmatrix}
    \otimes\begin{pmatrix}s_1^*+s_2^* & 0\\0 & s_1^*-s_2^*\end{pmatrix}}.
    \label{eq:CZ_unravel}
\end{equation}
One verifies that $\avgT{s_k(s_{k'}^* \pm s_{k''}^*)} = \delta_{kk'} \pm \delta_{kk''}$: the $+$ superposition gives unit average for both control states $\ket{0}$ and $\ket{1}$, while the $-$ superposition selectively introduces a $-1$ for the $\ket{11}$ component, reproducing the $\hat{Z}$ phase on the target. %Alternatively, $\hat{CZ} = (\hat{I}\otimes\hat{H})\,\hat{\mathrm{CNOT}}\,(\hat{I}\otimes\hat{H})$, so the unraveling follows directly from Eq.~(\ref{eq:CNOT_unravel_supp}) by conjugating the target-qubit signal matrix with the Hadamard.

\subsection{SWAP gate}
This gate permutes the two-qubit basis: $\hat{SWAP}\ket{ab} = \ket{ba}$. Its unitary matrix has non-zero off-diagonal blocks, requiring four distinct orthonormal signals $s_1,\ldots,s_4$:
\begin{equation}
    \hat{SWAP} = \avgT{\begin{pmatrix}s_1 & s_3\\s_4 & s_2\end{pmatrix}
    \otimes\begin{pmatrix}s_1^* & s_4^*\\s_3^* & s_2^*\end{pmatrix}}.
    \label{eq:SWAP_unravel}
\end{equation}
The cross terms average to zero by orthogonality ($\avgT{s_k s_{k'}^*}=\delta_{kk'}$), while each diagonal element $[S_1]_{\mu\nu}[S_2]_{\nu\mu}$ yields a matched $s_k s_k^*$ product with unit time average, reproducing every $1$ in the SWAP permutation matrix. %SWAP unraveling is used in the layer decomposition to connect non-adjacent qubits (Sec.~\ref{subsec:circuit_univ}).

\subsection{$\hat{R}_Y\otimes\hat{I}$ gate (passive)}
Up to now, we have shown two-wavebit gates that are actively passing on temporal dynamics to the wavebits. Here, we introduce a two-wavebit gate which rotates wavebit~1 about the $Y$-axis while leaving wavebit~2 unchanged. This example illustrates the concept of \emph{passive} gates which will serve as a building block for analog layer decomposition introduced in the main text.
\begin{equation}
    \hat{R}_Y(\theta)\otimes\hat{I}
    =\begin{pmatrix}\cos\tfrac{\theta}{2}&-\sin\tfrac{\theta}{2}\\
    \sin\tfrac{\theta}{2}&\cos\tfrac{\theta}{2}\end{pmatrix}
    \otimes
    \begin{pmatrix}1&0\\0&1\end{pmatrix}.
    \label{eq:Ry_gate}
\end{equation}
Because it is separable, it is implemented as a \emph{static} matrix acting independently on the channels $[\alpha_0^{(1)},\alpha_1^{(1)}]$ of wavebit~1 and $[\alpha_0^{(2)},\alpha_1^{(2)}]$ of wavebit~2, with all signal amplitudes held at their constant (DC) values. No oscillating signals are required: the base frequency is $\Omega=0$ and the time average is trivially satisfied for any window $T$. Note that rotations about other axes ($R_X$, $R_Z$, or arbitrary $SU(2)$ unitaries paired with an identity) are achieved identically — only the constant matrix entries change.

\newpage
% ============================================================
% ============================================================
\section{System Design and Implementation}
\label{sup:sec:S_hardware_design}
% ============================================================

The design goal of the two-wavebit analog prototype is to emulate 2-qubit circuits of the form $(\hat{C}_1\otimes\hat{C}_2)\cdot\hat{\mathrm{CNOT}}$ — two independent single-qubit gates followed by a single CNOT — with the Bell State Generation Circuit (BSGC, Fig.~\ref{fig:S_bsgc_intro}) as the minimum design target.  The implementation is restricted to real probability amplitudes; extension to complex coefficients is possible in analog electronics by representing real and imaginary parts as separate voltages, but was not required here.

\begin{figure}[htbp]
\centering
\scalebox{0.75}{\input{figures/BSGC_pdb}}
\caption{\textbf{Bell State Generation Circuit (BSGC).} Minimum design target: for each computational basis input the circuit produces one of the four maximally entangled Bell states.}
\label{fig:S_bsgc_intro}
\end{figure}

\subsection{System Overview}

Although the formalism allows unraveling an entire 2-qubit circuit in one step, doing so for each individual 2-qubit gate (as implemented here) is the scalable approach: it keeps the required number of base frequencies scaling linearly with the number of entangling layers, $\mathcal{O}(\delta)$.  The emulator therefore contains two layers: first, a layer of two static single-qubit gates $\hat{C}_1$, $\hat{C}_2$ applied in parallel; and second, a layer implementing the unraveled $\hat{\mathrm{CNOT}}$ gate via time-varying signals.  After these layers the tensor product and time average must be applied explicitly to read the result.  The implemented circuit is summarized in Fig.~\ref{fig:S_board_circuit}.

\begin{figure}[htbp]
\centering
\resizebox{0.6\linewidth}{!}{\input{figures/Processing_Board_Circuit_Scheme}}
\caption{\textbf{Main operations implemented by the emulator.} Static single-qubit layers $\hat{C}_1$, $\hat{C}_2$ are applied first; the time-varying CNOT layer $\hat{S}_1(t)\otimes\hat{S}_2(t)$ follows; tensor product and time-averaging complete the computation.}
\label{fig:S_board_circuit}
\end{figure}

Each qubit is represented by two voltages in $[-10\,\mathrm{V},+10\,\mathrm{V}]$; each voltage IS one of the two probability amplitudes of the qubit.  The machine unit is $10\,\mathrm{V}$, mapping onto the mathematical range $[-1,+1]$.  Initial qubit states and the coefficients of $\hat{C}_1$, $\hat{C}_2$ are user-adjustable via potentiometers.  The time-dependent signals $\hat{S}_1(t)$, $\hat{S}_2(t)$ — implementing the unraveled CNOT — are generated by a dedicated \textit{Signal Board} PCB whose waveforms are programmed by a microcontroller.  The output is displayed after the time-averaging step via four pairs of LEDs.

The system is split into two PCBs — \textit{Signal Board} and \textit{Processing Board} — so that the Signal Board (the least modular component, currently implementing only the CNOT) can be replaced or extended to implement other gate layers without changing the Processing Board.  The computational stages of each board are shown in Figs.~\ref{fig:S_signal_flowchart} and~\ref{fig:S_proc_flowchart}.

\subsection{Signal Board}
\label{sup:sec:S_signal_board}

\begin{figure}[htbp]
\centering
\includegraphics[width=0.5\linewidth]{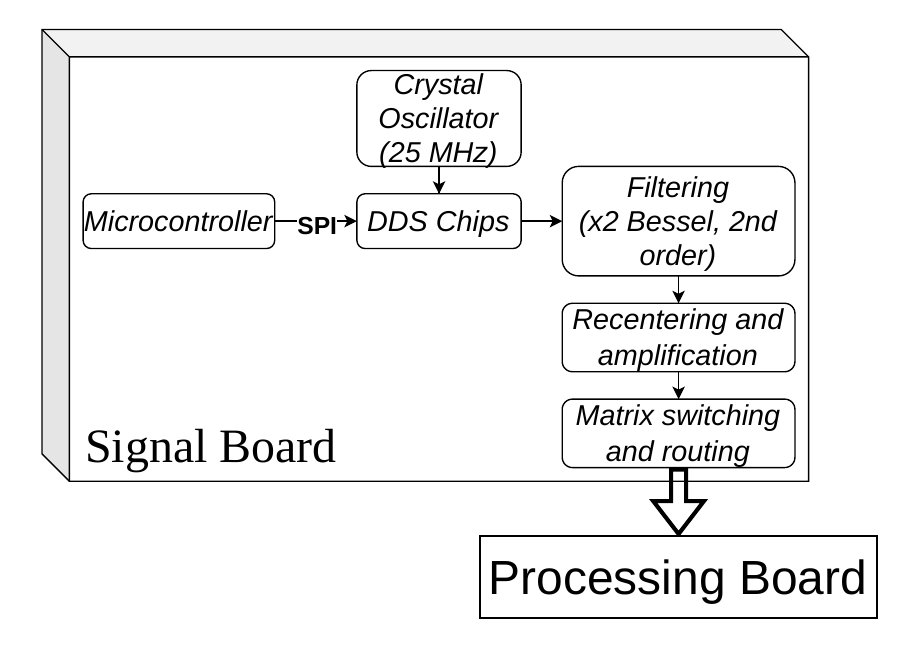}
\caption{\textbf{Signal Board flowchart.} The two carrier signals are synthesized by DDS chips, low-pass filtered (Bessel, $f_c=101\,\mathrm{kHz}$), recentered and amplified to the $10\,\mathrm{V}$ machine unit, then routed and switched to the eight matrix-element output lines.}
\label{fig:S_signal_flowchart}
\end{figure}

\subsubsection{Objective}

The $\hat{\mathrm{CNOT}}$ gate has only four non-zero entries, which allows a particularly compact unraveling using just two orthonormal signals $\{s_1(t),s_2(t)\}$ — far fewer than the sixteen required by the general construction of Appendix~\ref{app:gate_expand} of the main text:
\begin{equation}
\hat{\mathrm{CNOT}} = \avgT{\begin{pmatrix}s_1(t) & 0 \\ 0 & s_2(t)\end{pmatrix}
\otimes\begin{pmatrix}s_1(t) & s_2(t) \\ s_2(t) & s_1(t)\end{pmatrix}}.
\end{equation}
The goal of the Signal Board is to generate these two orthonormal signals.

\subsubsection{Signal generation}

The signals are generated by Direct Digital Synthesis (DDS): the AD9833 chips are essentially programmable DACs that output a sinusoid at a frequency set via SPI.  The Signal Board is a true mixed-signal design, combining a digital microcontroller, SPI communication, DACs, and analog processing.  DDS was chosen over fully analog oscillators because maintaining a constant relative phase between two analog oscillators requires complex control loops, whereas two DDS chips sharing the same external crystal oscillator track phase coherently by construction.  Constant relative phase is critical here because it directly preserves the orthogonality of $s_1$ and $s_2$.  SPI communication occurs only once at power-on to program the frequencies; there is no digital switching noise thereafter.

\subsubsection{Analog signal conditioning}

The raw AD9833 output has a DC offset of $344\,\mathrm{mV}$ and an amplitude of only $306\,\mathrm{mV}$, whereas the requirement is zero DC offset and an amplitude equal to the machine unit of $10\,\mathrm{V}$.  A precision $2.048\,\mathrm{V}$ reference is divided down to $343.8\,\mathrm{mV}$ and subtracted from the DDS output; the result is then amplified by a factor of $32.5$.  The final signal has a negligible DC offset of $\approx6.5\,\mathrm{mV}$ and an amplitude of $\approx9.95\,\mathrm{V}$ (Fig.~\ref{fig:S_dds_recenter}).

To remove residual digital switching noise while preserving the relative phase between the two carriers, a 2nd-order Bessel low-pass filter ($f_c=101\,\mathrm{kHz}$, Sallen--Key topology, Fig.~\ref{fig:S_sallen_key}) is placed at each DDS output.  Bessel filters have maximally flat group delay, so both carriers experience identical phase shifts, maintaining their orthogonality through the filter.

\begin{figure}[htbp]
\centering
\includegraphics[width=0.6\linewidth]{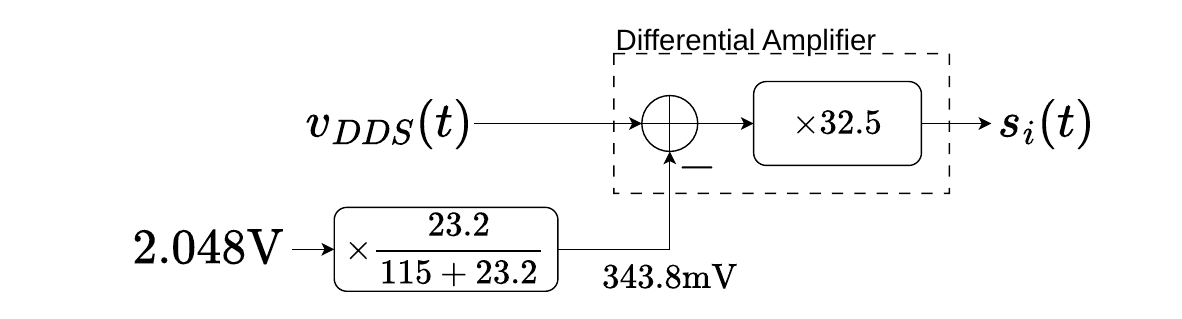}
\caption{\textbf{DDS output recentering and amplification.} A precision voltage reference removes the $344\,\mathrm{mV}$ DC offset; a subsequent gain of $32.5$ raises the amplitude to the $10\,\mathrm{V}$ machine unit.}
\label{fig:S_dds_recenter}
\end{figure}

\begin{figure}[htbp]
\centering
\resizebox{0.5\linewidth}{!}{\input{figures/sallen_key_topology_pdb}}
\caption{\textbf{Sallen--Key low-pass filter topology} used on the Signal Board ($f_c=101\,\mathrm{kHz}$, 2nd-order Bessel) and on the Processing Board for time-averaging ($f_c\approx2\,\mathrm{Hz}$, 2nd-order critically damped).}
\label{fig:S_sallen_key}
\end{figure}

\subsubsection{Routing and switching}

The conditioned signals are buffered and routed into eight output traces corresponding to the elements of both $\hat{S}_i(t)$ matrices.  Before the switches, the routing implements:
\begin{equation}
\hat{S}_1'(t) = \begin{pmatrix}s_1(t) & s_2(t) \\ s_1(t) & s_2(t)\end{pmatrix}, \qquad
\hat{S}_2'(t) = \begin{pmatrix}s_1(t) & s_2(t) \\ s_2(t) & s_1(t)\end{pmatrix}.
\end{equation}
A set of eight switches allows the user to force any matrix element to true zero.  In particular, zeroing the off-diagonal components of $\hat{S}_1'$ yields the CNOT unraveling (diagonal $\hat{S}_1$, full $\hat{S}_2$).

\subsection{Processing Board}
\label{sup:sec:S_proc_board}

\begin{figure}[htbp]
\centering
\includegraphics[width=0.8\linewidth]{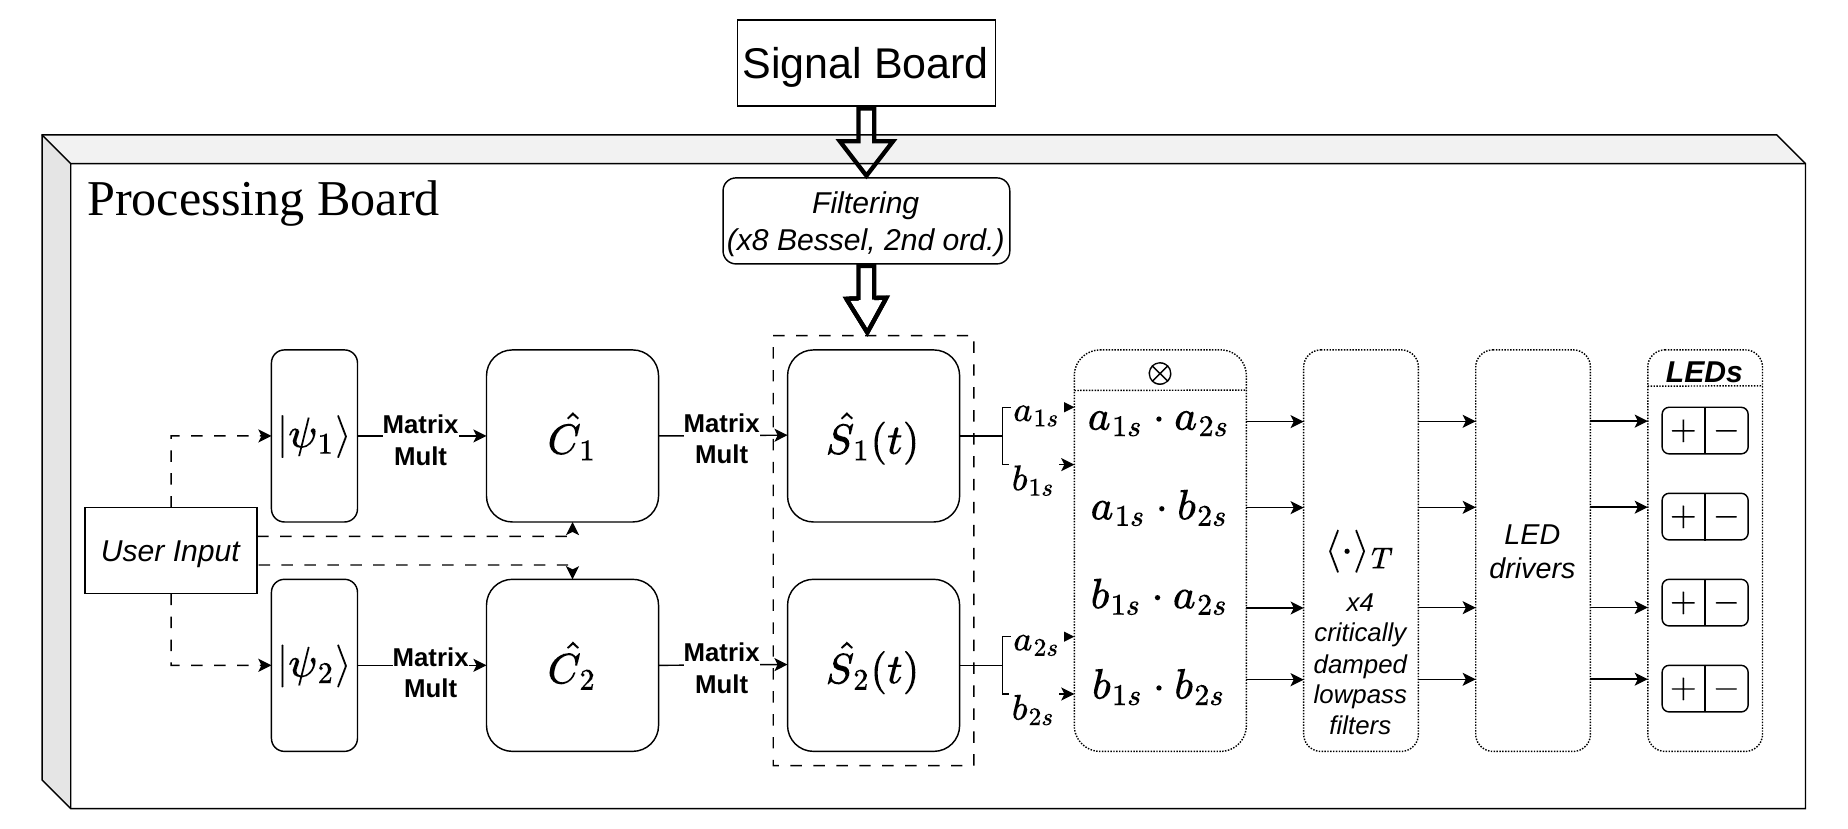}
\caption{\textbf{Processing Board flowchart.} Qubit states are encoded via bVGAs from a $10\,\mathrm{V}$ reference; a second bVGA stage applies $\hat{C}_1$, $\hat{C}_2$; AD633 ICs multiply in the time-varying CNOT signals; four AD633s compute the tensor product; a $2\,\mathrm{Hz}$ Sallen--Key filter time-averages; LED pairs display the output.}
\label{fig:S_proc_flowchart}
\end{figure}

\subsubsection{Power}

The entire setup is powered by USB-C. The power delivery network converts and regulates the bus voltage into all rails required by the digital (microcontroller, DDS) and analog ($\pm10\,\mathrm{V}$, precision reference) subsystems of both boards, as shown in Fig.~\ref{fig:S_power}.

\begin{figure}[htbp]
\centering
\includegraphics[width=0.8\linewidth]{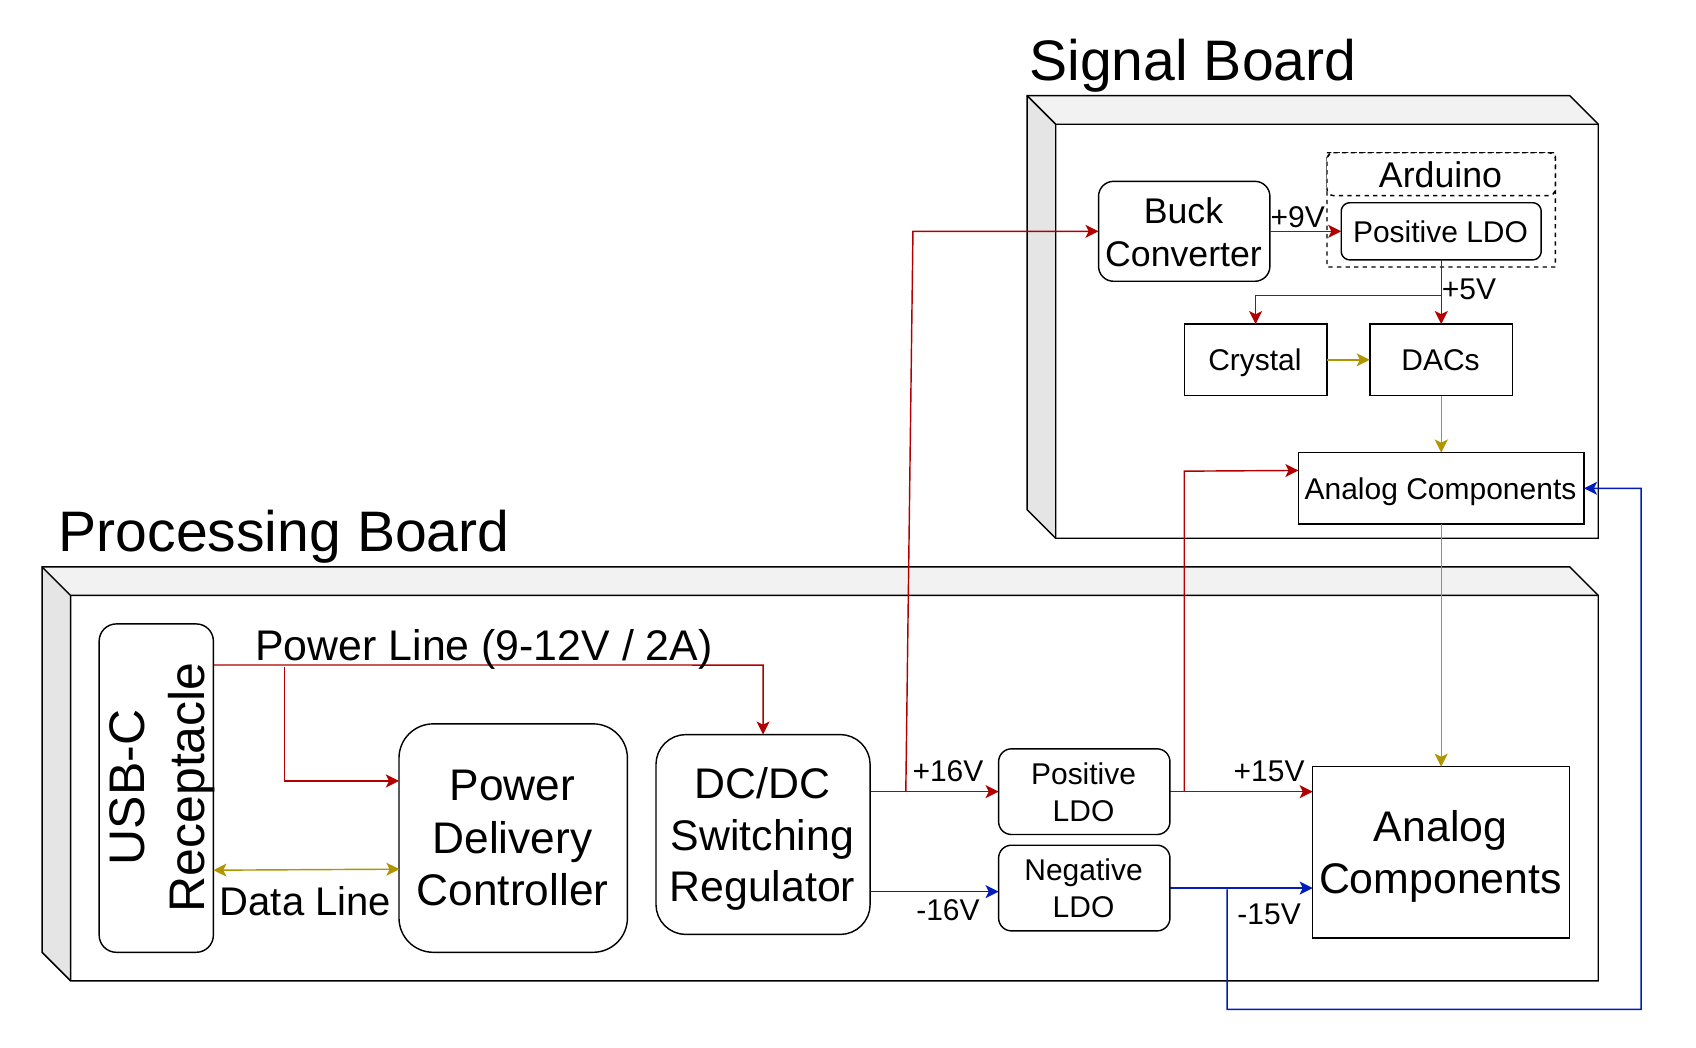}
\caption{\textbf{Power system flowchart.} USB-C input is regulated and distributed to all digital and analog subsystems.}
\label{fig:S_power}
\end{figure}

\subsubsection{User input}
\label{sup:sec:S_user_input}

The user input is fully analog.  Using a bipolar Variable Gain Amplifier (bVGA, Fig.~\ref{fig:S_bVGA}), the user can multiply any input voltage by a factor in $[-1,+1]$.  A first set of bVGAs is connected to a $10\,\mathrm{V}$ reference so that the user selects the initial probability amplitudes of each qubit.  A second set of bVGAs is daisy-chained immediately after — two per qubit element — and implements the matrix coefficients of $\hat{C}_1$ and $\hat{C}_2$.  In total, 12 bVGAs constitute the primary user interface of the board.

\begin{figure}[htbp]
\centering
\resizebox{0.45\linewidth}{!}{\input{figures/bVGA_pdb}}
\caption{\textbf{Bipolar Variable Gain Amplifier (bVGA)} topology ($\alpha\in[-1,+1]$).  Used for both qubit-state encoding (from $10\,\mathrm{V}$ reference) and single-qubit matrix element selection.}
\label{fig:S_bVGA}
\end{figure}

Because analog potentiometers are difficult to set precisely, ``True~0'' switches are added to force any output directly to ground (a true 0 via bVGA requires the potentiometer to be at exactly half rotation).  At the matrix-element level, an additional set of switches enables multiplication by $1/\sqrt{2}$, a common value in Hadamard gates that is equally impractical to set by potentiometer.

\subsubsection{Signal input}

The Signal Board sits as a ``hat board'' on top of the Processing Board.  The Processing Board includes a second stage of eight 2nd-order Bessel low-pass filters (same specifications as those on the Signal Board, $f_c=101\,\mathrm{kHz}$) to further attenuate any noise on the carrier lines and to ease future Signal Board replacement.

\subsubsection{Matrix multiplication and tensor product}

Matrix multiplication is implemented differently for the static and time-varying matrices.  In both cases the computation reduces to element-wise multiplication followed by summation; the summation stage is a standard inverter-summer topology (Fig.~\ref{fig:S_inv_sum}) for both.

\begin{figure}[htbp]
\centering
\resizebox{0.45\linewidth}{!}{\input{figures/inverter_summer_pdb}}
\caption{\textbf{Inverter-summer topology} used for the summation stage of both static and dynamic matrix multiplications.}
\label{fig:S_inv_sum}
\end{figure}

For the static matrices $\hat{C}_1$, $\hat{C}_2$, the multiplication is already performed by the bVGAs (Sec.~\ref{sup:sec:S_user_input}).  For the time-varying signals $\hat{S}_1(t)$, $\hat{S}_2(t)$, an AD633 four-quadrant analog multiplier IC is used to multiply each signal element into the corresponding qubit coefficient.

The two-qubit tensor product is then computed by four further AD633 multiplications:
\begin{equation}
\begin{pmatrix}a_{1s} \\ b_{1s}\end{pmatrix}
\otimes
\begin{pmatrix}a_{2s} \\ b_{2s}\end{pmatrix}
=
\begin{pmatrix}a_{1s}a_{2s} \\ a_{1s}b_{2s} \\ b_{1s}a_{2s} \\ b_{1s}b_{2s}\end{pmatrix}.
\end{equation}
A labeling convention in the board schematic results in the physical implementation of $|\psi_2\rangle\otimes|\psi_1\rangle$ rather than $|\psi_1\rangle\otimes|\psi_2\rangle$; this corresponds to the Qiskit little-endian convention and does not affect the validity of the computation.

\subsubsection{Averaging and LEDs}

To recover the DC value of the tensor-product signals, a 2nd-order critically damped low-pass filter with $f_c\approx2\,\mathrm{Hz}$ (Sallen--Key topology, Fig.~\ref{fig:S_sallen_key}) is applied to each of the four outputs.  This implements the time-averaging operation $\langle\cdot\rangle_T$.

Each averaged output is then fed into an LED Driver circuit (Fig.~\ref{fig:S_led_driver}) capable of driving two LEDs connected in anti-parallel.  The LED that lights up depends on the sign of the input voltage: a green LED indicates a positive probability amplitude and a red LED indicates a negative value.  The circuit handles the differing forward voltages of the two LED colors, avoids dead zones for inputs below the forward voltage, and scales brightness linearly with the input magnitude.

\begin{figure}[htbp]
\centering
\resizebox{0.3\linewidth}{!}{\input{figures/LED_drivers_pdb}}
\caption{\textbf{LED driver circuit.} Anti-parallel green (positive) and red (negative) LEDs display the sign and magnitude of each time-averaged output amplitude; the circuit handles differing forward voltages and avoids dead zones.}
\label{fig:S_led_driver}
\end{figure}

\newpage
% ============================================================
\section{Experimental Validation}
\label{sup:sec:S_experimental}
% ============================================================

\subsection{Hardware Normalization and Measurement Notes}
\label{sup:sec:S7_hardware}

\textit{Machine unit.}  The analog processing board operates with a peak
voltage of $10\,\mathrm{V}$.  All output voltages are therefore normalized by $10\,\mathrm{V}$ to map onto $[-1,1]$.\\

\textit{Tensor product normalization.}  An error in the processing board causes
the tensor product output to be normalized by $1/\sqrt{2}$ instead of 1. Accounting for this, the reported experimental values are normalized by $10\,\mathrm{V}/\sqrt{2} \approx 7.07\,\mathrm{V}$.  All tables in the main text use this normalization consistently.\\

\textit{Phase kickback oscillations.}  Low-frequency ($\sim10\,\mathrm{mHz}$)
oscillations observed under the phase kickback input conditions (Fig.~4 of main text) are attributed to a nonlinearity in the analog multiplier chain under conditions where the two input signal frequencies produce near-DC beat frequencies through higher-order mixing.  The exact mechanism is under investigation; the oscilloscope digital average eliminates this artifact, as the oscillation period ($\sim100\,\mathrm{s}$) is much longer than the $2\,\mathrm{Hz}$ cutoff of the averaging filter.\\

\textit{Multimeter vs.\ oscilloscope.}  For all circuits except phase kickback,
the post-filter DC values were read with a standard digital multimeter.  For phase kickback, an oscilloscope with a $2\,\mathrm{s}/\mathrm{div}$ time division was used to compute the digital time-average, excluding the slow oscillation artifact.

\subsection{Detailed Experimental Results}
\label{sup:sec:S9_analog}

This section presents full measurement tables for all six circuits tested on the two-wavebit analog prototype.
The hardware design and signal-conditioning details are described in Sec.~\ref{sup:sec:S_hardware_design}; output normalization conventions are described in Sec.~\ref{sup:sec:S7_hardware}.
Each circuit was implemented by setting the static encoding matrices $\hat{C}_1$, $\hat{C}_2$ and the initial qubit amplitudes via potentiometers.
The Signal Board supplied two sinusoidal carriers at $f_1=1\,\mathrm{kHz}$ and $f_2=3\,\mathrm{kHz}$.
In each table, \textit{Th.}\ denotes the ideal target amplitude from IBM's Quantum Composer and \textit{Meas.}\ the normalized DC voltage measured at the board output.
State labels $|ij\rangle$ follow Qiskit's little-endian convention: $|\psi_2{=}i,\psi_1{=}j\rangle$, where $\psi_1$ is the control qubit and $\psi_2$ the target.

Because the prototype is a first-generation proof-of-concept, success is assessed by three criteria rather than a single quantitative threshold:
\begin{itemize}
  \item \textit{State topology}: outputs that should be zero (in theory) are in the tens of millivolts; outputs that should be non-zero are clearly non-negligible.
  \item \textit{Phase parity}: each non-zero output has the correct sign.
  \item \textit{Amplitude ordering}: when two or more outputs are non-zero, their relative magnitudes are ordered as predicted.
\end{itemize}
The four computational basis inputs $|\psi_1\rangle|\psi_2\rangle \in \{|0\rangle|0\rangle, |0\rangle|1\rangle, |1\rangle|0\rangle, |1\rangle|1\rangle\}$ were tested for every circuit, since a circuit is uniquely characterized by its action on any basis of the space.

\subsubsection{Pure CNOT}
\label{subsec:S9_cnot}

\begin{figure}[htbp]
\centering
\scalebox{0.75}{\input{figures/CNOT_pdb}}
\caption{\textbf{Pure CNOT circuit.} Tests the Signal Board and tensor-product stage independently of the single-qubit encoding layer.}
\label{fig:S_cnot}
\end{figure}

The CNOT gate (Fig.~\ref{fig:S_cnot}) was tested for all four computational basis inputs and additionally for the phase-kickback input $|\!+\rangle|\!-\rangle$, since $\hat{\mathrm{CNOT}}|{+}\rangle|{-}\rangle = |{-}\rangle|{-}\rangle$ is an important quantum-computing primitive.
For the four basis inputs the average absolute error is 0.012 (maximum 0.026).
The phase-kickback setup exhibits slightly larger errors (average 0.035, maximum 0.047) due to the slow spurious oscillations described in Sec.~\ref{sup:sec:S7_hardware}; an oscilloscope digital average recovers the correct DC value.
In all five cases state topology, phase parity, and amplitude ordering are correct.

\begin{table}[htbp]
\centering
\caption{\textbf{CNOT: theoretical vs.\ measured output amplitudes.}
Normalized measured DC voltages (see Sec.~\ref{sup:sec:S7_hardware}) compared to the ideal statevector.
The phase-kickback row $|{+}\rangle|{-}\rangle$ was read with an oscilloscope digital average (see Sec.~\ref{sup:sec:S7_hardware}).}
\label{tab:S_cnot}
\begin{ruledtabular}
\begin{tabular}{lcccccccc}
 & \multicolumn{2}{c}{$|00\rangle$} & \multicolumn{2}{c}{$|01\rangle$}
 & \multicolumn{2}{c}{$|10\rangle$} & \multicolumn{2}{c}{$|11\rangle$} \\
Input & Th. & Meas. & Th. & Meas. & Th. & Meas. & Th. & Meas. \\
\hline
$|0\rangle|0\rangle$ & $1$    & $0.98$ & $0$     & $0.00$ & $0$      & $0.00$  & $0$     & $0.00$ \\
$|0\rangle|1\rangle$ & $0$    & $0.00$ & $0$     & $0.00$ & $1$      & $0.98$  & $0$     & $0.00$ \\
$|1\rangle|0\rangle$ & $0$    & $0.00$ & $0$     & $0.00$ & $0$      & $0.00$  & $1$     & $0.99$ \\
$|1\rangle|1\rangle$ & $0$    & $0.00$ & $1$     & $0.97$ & $0$      & $0.00$  & $0$     & $0.00$ \\
\hline
$|{+}\rangle|{-}\rangle$ & $\phantom{-}0.5$ & $\phantom{-}0.45$ & $-0.5$ & $-0.52$ & $-0.5$ & $-0.52$ & $\phantom{-}0.5$ & $\phantom{-}0.45$ \\
\end{tabular}
\end{ruledtabular}
\end{table}

\subsubsection{Bell State Generation Circuit}
\label{subsec:S9_bsgc}

\begin{figure}[htbp]
\centering
\scalebox{0.75}{\input{figures/BSGC_pdb}}
\caption{\textbf{Bell State Generation Circuit (BSGC).} For each computational basis input, the circuit produces one of the four maximally entangled Bell states.}
\label{fig:S_bsgc}
\end{figure}

The BSGC (Fig.~\ref{fig:S_bsgc}) applies $\hat{H}$ to qubit~$\psi_1$ via $\hat{C}_1 = \hat{H}$, with $\hat{C}_2 = \hat{I}$, followed by the unraveled CNOT layer.
This test verifies whether the emulator can represent maximally entangled states.
Average absolute error is 0.007 (maximum 0.021), confirming accurate emulation of all four Bell states.

\begin{table}[htbp]
\centering
\caption{\textbf{BSGC: theoretical vs.\ measured output amplitudes.}
Each row corresponds to one of the four Bell states produced by the circuit.}
\label{tab:S_bsgc}
\begin{ruledtabular}
\begin{tabular}{lcccccccc}
 & \multicolumn{2}{c}{$|00\rangle$} & \multicolumn{2}{c}{$|01\rangle$}
 & \multicolumn{2}{c}{$|10\rangle$} & \multicolumn{2}{c}{$|11\rangle$} \\
Input & Th. & Meas. & Th. & Meas. & Th. & Meas. & Th. & Meas. \\
\hline
$|0\rangle|0\rangle$ & $\phantom{-}0.707$ & $\phantom{-}0.69$ & $0$      & $0.00$ & $0$     & $0.00$ & $\phantom{-}0.707$ & $\phantom{-}0.69$ \\
$|0\rangle|1\rangle$ & $0$                & $0.00$            & $\phantom{-}0.707$ & $\phantom{-}0.69$ & $\phantom{-}0.707$ & $\phantom{-}0.69$ & $0$ & $0.00$ \\
$|1\rangle|0\rangle$ & $\phantom{-}0.707$ & $\phantom{-}0.70$ & $0$      & $0.00$ & $0$     & $0.00$ & $-0.707$           & $-0.70$ \\
$|1\rangle|1\rangle$ & $0$                & $0.00$            & $-0.707$ & $-0.69$ & $\phantom{-}0.707$ & $\phantom{-}0.69$ & $0$ & $0.00$ \\
\end{tabular}
\end{ruledtabular}
\end{table}

\subsubsection{Double Hadamard into CNOT}
\label{subsec:S9_doubleH}

\begin{figure}[htbp]
\centering
\scalebox{0.75}{\input{figures/double_H_pdb}}
\caption{\textbf{Double-Hadamard circuit.} Both qubits pass through $\hat{H}$ before the CNOT layer, producing a four-component output state and exercising all tensor-product channels simultaneously.}
\label{fig:S_doubleH}
\end{figure}

With $\hat{C}_1 = \hat{C}_2 = \hat{H}$ (Fig.~\ref{fig:S_doubleH}), all four output amplitudes are non-zero simultaneously, providing a stringent test of the full tensor-product stage.
Average absolute error is 0.043 (maximum 0.059) — noticeably higher than other circuits because every output channel exhibits the slow spurious oscillations (see Sec.~\ref{sup:sec:S7_hardware}).
Nonetheless, state topology, phase parity, and amplitude ordering are preserved in all cases.

\begin{table}[htbp]
\centering
\caption{\textbf{Double-Hadamard CNOT: theoretical vs.\ measured output amplitudes.}
All four output amplitudes are non-zero, so all channels are stressed simultaneously.}
\label{tab:S_doubleH}
\begin{ruledtabular}
\begin{tabular}{lcccccccc}
 & \multicolumn{2}{c}{$|00\rangle$} & \multicolumn{2}{c}{$|01\rangle$}
 & \multicolumn{2}{c}{$|10\rangle$} & \multicolumn{2}{c}{$|11\rangle$} \\
Input & Th. & Meas. & Th. & Meas. & Th. & Meas. & Th. & Meas. \\
\hline
$|0\rangle|0\rangle$ & $\phantom{-}0.5$ & $\phantom{-}0.45$ & $\phantom{-}0.5$ & $\phantom{-}0.44$ & $\phantom{-}0.5$ & $\phantom{-}0.45$ & $\phantom{-}0.5$ & $\phantom{-}0.45$ \\
$|0\rangle|1\rangle$ & $\phantom{-}0.5$ & $\phantom{-}0.45$ & $-0.5$ & $-0.52$ & $-0.5$ & $-0.53$ & $\phantom{-}0.5$ & $\phantom{-}0.45$ \\
$|1\rangle|0\rangle$ & $\phantom{-}0.5$ & $\phantom{-}0.45$ & $-0.5$ & $-0.53$ & $\phantom{-}0.5$ & $\phantom{-}0.45$ & $-0.5$ & $-0.53$ \\
$|1\rangle|1\rangle$ & $\phantom{-}0.5$ & $\phantom{-}0.45$ & $\phantom{-}0.5$ & $\phantom{-}0.44$ & $-0.5$ & $-0.53$ & $-0.5$ & $-0.53$ \\
\end{tabular}
\end{ruledtabular}
\end{table}

\subsubsection{Bloch-sphere rotations: fractional entanglement}
\label{subsec:S9_frac}

\begin{figure}[htbp]
\centering
\scalebox{0.75}{\input{figures/rotations1_pdb}}
\caption{\textbf{Fractional-entanglement circuit.} $\hat{R}_Y(\pi/3)$ on qubit $\psi_1$ followed by CNOT, producing partially entangled states with unequal amplitudes.}
\label{fig:S_frac}
\end{figure}

With $\hat{C}_1 = \hat{R}_Y(\pi/3)$ and $\hat{C}_2 = \hat{I}$ (Fig.~\ref{fig:S_frac}), the circuit produces partially entangled output states.
This test verifies whether the emulator can represent non-maximally entangled states with unequal amplitude ratios ($\sqrt{3}/2$ vs.\ $1/2$).
Average absolute error is 0.005 (maximum 0.017), the lowest across all tested circuits.

\begin{table}[htbp]
\centering
\caption{\textbf{Fractional-entanglement circuit: theoretical vs.\ measured output amplitudes.}
$\hat{C}_1=\hat{R}_Y(\pi/3)$, $\hat{C}_2=\hat{I}$.}
\label{tab:S_frac}
\begin{ruledtabular}
\begin{tabular}{lcccccccc}
 & \multicolumn{2}{c}{$|00\rangle$} & \multicolumn{2}{c}{$|01\rangle$}
 & \multicolumn{2}{c}{$|10\rangle$} & \multicolumn{2}{c}{$|11\rangle$} \\
Input & Th. & Meas. & Th. & Meas. & Th. & Meas. & Th. & Meas. \\
\hline
$|0\rangle|0\rangle$ & $\phantom{-}0.866$ & $\phantom{-}0.85$ & $0$      & $0.00$ & $0$      & $0.00$ & $\phantom{-}0.5$ & $\phantom{-}0.49$ \\
$|0\rangle|1\rangle$ & $0$                & $0.00$            & $\phantom{-}0.5$ & $\phantom{-}0.49$ & $\phantom{-}0.866$ & $\phantom{-}0.86$ & $0$ & $0.00$ \\
$|1\rangle|0\rangle$ & $-0.5$             & $-0.50$           & $0$      & $0.00$ & $0$      & $0.00$ & $\phantom{-}0.866$ & $\phantom{-}0.86$ \\
$|1\rangle|1\rangle$ & $0$                & $0.00$            & $\phantom{-}0.866$ & $\phantom{-}0.85$ & $-0.5$ & $-0.50$ & $0$ & $0.00$ \\
\end{tabular}
\end{ruledtabular}
\end{table}

\subsubsection{Bloch-sphere rotations: asymmetric tensor product}
\label{subsec:S9_asym}

\begin{figure}[htbp]
\centering
\scalebox{0.75}{\input{figures/rotations2_pdb}}
\caption{\textbf{Asymmetric tensor-product circuit.} $\hat{R}_Y(\pi/2)$ on $\psi_1$ and $\hat{R}_Y(\pi)$ on $\psi_2$ before CNOT, testing independent non-identity single-qubit operations on both qubits.}
\label{fig:S_asym}
\end{figure}

With $\hat{C}_1 = \hat{R}_Y(\pi/2)$ and $\hat{C}_2 = \hat{R}_Y(\pi)$ (Fig.~\ref{fig:S_asym}), both qubits undergo different non-identity rotations before the CNOT.
This verifies whether independent, asymmetric single-qubit operations are handled correctly by the encoding stage.
Average absolute error is 0.009 (maximum 0.023).

\begin{table}[htbp]
\centering
\caption{\textbf{Asymmetric tensor-product circuit: theoretical vs.\ measured output amplitudes.}
$\hat{C}_1=\hat{R}_Y(\pi/2)$, $\hat{C}_2=\hat{R}_Y(\pi)$.}
\label{tab:S_asym}
\begin{ruledtabular}
\begin{tabular}{lcccccccc}
 & \multicolumn{2}{c}{$|00\rangle$} & \multicolumn{2}{c}{$|01\rangle$}
 & \multicolumn{2}{c}{$|10\rangle$} & \multicolumn{2}{c}{$|11\rangle$} \\
Input & Th. & Meas. & Th. & Meas. & Th. & Meas. & Th. & Meas. \\
\hline
$|0\rangle|0\rangle$ & $0$      & $0.00$ & $\phantom{-}0.707$ & $\phantom{-}0.68$ & $\phantom{-}0.707$ & $\phantom{-}0.69$ & $0$      & $0.00$ \\
$|0\rangle|1\rangle$ & $-0.707$ & $-0.69$ & $0$               & $0.00$            & $0$               & $0.00$            & $-0.707$ & $-0.69$ \\
$|1\rangle|0\rangle$ & $0$      & $0.00$ & $\phantom{-}0.707$ & $\phantom{-}0.69$ & $-0.707$          & $-0.69$           & $0$      & $0.00$ \\
$|1\rangle|1\rangle$ & $\phantom{-}0.707$ & $\phantom{-}0.69$ & $0$ & $0.00$ & $0$ & $0.00$ & $-0.707$ & $-0.69$ \\
\end{tabular}
\end{ruledtabular}
\end{table}

\subsubsection{Reflection test}
\label{subsec:S9_refl}

\begin{figure}[htbp]
\centering
\scalebox{0.75}{\input{figures/reflection_pdb}}
\caption{\textbf{Reflection circuit.} $\hat{M}(53.1^\circ)$ on $\psi_1$ followed by CNOT.
$\hat{M}$ has $\det(\hat{M})=-1$, testing whether the emulator correctly handles reflections.}
\label{fig:S_refl}
\end{figure}

With $\hat{C}_1 = \hat{M}(53.1^\circ)$ and $\hat{C}_2 = \hat{I}$ (Fig.~\ref{fig:S_refl}), where
\begin{equation}
\hat{M}(\theta) = \begin{pmatrix}\cos\theta & \sin\theta \\ \sin\theta & -\cos\theta\end{pmatrix},
\end{equation}
the circuit tests a gate with $\det(\hat{M})=-1$.
All previous circuits used gates with positive determinant (proper rotations); this test verifies whether the emulator also handles improper rotations (reflections) correctly.
For $\theta\approx53.1^\circ$, one gets $\cos\theta=0.6$ and $\sin\theta=0.8$, yielding simple rational coefficients.
Average absolute error is 0.006 (maximum 0.018).

\begin{table}[htbp]
\centering
\caption{\textbf{Reflection circuit: theoretical vs.\ measured output amplitudes.}
$\hat{C}_1=\hat{M}(53.1^\circ)$, $\hat{C}_2=\hat{I}$, $\cos(53.1^\circ)=0.6$, $\sin(53.1^\circ)=0.8$.}
\label{tab:S_refl}
\begin{ruledtabular}
\begin{tabular}{lcccccccc}
 & \multicolumn{2}{c}{$|00\rangle$} & \multicolumn{2}{c}{$|01\rangle$}
 & \multicolumn{2}{c}{$|10\rangle$} & \multicolumn{2}{c}{$|11\rangle$} \\
Input & Th. & Meas. & Th. & Meas. & Th. & Meas. & Th. & Meas. \\
\hline
$|0\rangle|0\rangle$ & $\phantom{-}0.6$ & $\phantom{-}0.59$ & $0$      & $0.00$ & $0$     & $0.00$ & $\phantom{-}0.8$ & $\phantom{-}0.79$ \\
$|0\rangle|1\rangle$ & $0$              & $0.00$            & $\phantom{-}0.8$ & $\phantom{-}0.78$ & $\phantom{-}0.6$ & $\phantom{-}0.59$ & $0$ & $0.00$ \\
$|1\rangle|0\rangle$ & $\phantom{-}0.8$ & $\phantom{-}0.79$ & $0$      & $0.00$ & $0$     & $0.00$ & $-0.6$           & $-0.59$ \\
$|1\rangle|1\rangle$ & $0$              & $0.00$            & $-0.6$   & $-0.59$ & $\phantom{-}0.8$ & $\phantom{-}0.79$ & $0$ & $0.00$ \\
\end{tabular}
\end{ruledtabular}
\end{table}

\subsubsection{Discussion}
\label{subsec:S9_disc}

In every tested circuit, state topology and phase parity were exactly as expected.
Amplitude ordering was also always correct for cases where amplitudes were distinguishable.
For equiprobable cases (e.g.\ Bell states with $|\alpha|=1/\sqrt{2}$ for two outputs), the absolute error never exceeded 0.06.
The worst-performing circuit (double-Hadamard into CNOT) is entirely explained by the slow spurious oscillation described in Sec.~\ref{sup:sec:S7_hardware}: all four output channels showed the LFO artifact simultaneously, increasing every error by approximately $0.04$; the state topology, sign, and ordering remained unaffected.
For the remaining five circuits, errors are consistent with a combination of potentiometer-setting uncertainty and residual attenuation from the $2\,\mathrm{Hz}$ low-pass averaging filter (which may not reach full DC for low-amplitude AC components near cutoff).

\newpage
% ============================================================
\section{Digital Simulation: Convergence Analysis}
\label{sup:sec:S_convergence}
% ============================================================

\subsection{Beat-frequency threshold}

The finite-time error bound (Appendix~\ref{app:thm2} of the main text) guarantees that the fidelity $\mathcal{F}=|\langle\psi_q|\Psi_w\rangle|^2$ between the exact quantum output $|\psi_q\rangle$ and the time-averaged wavebit state $|\Psi_w\rangle$ converges as $\mathcal{O}(1/T)$ once $T$ exceeds the \emph{convergence timescale} $T^*=2\pi/\omega^*$, where
\begin{equation}
    \omega^*_\delta = \min_{\mathbf{k}\neq\mathbf{0}}
    \left|\sum_{\ell} k_\ell\,\Omega_\ell\right|
    \label{eq:omegastar}
\end{equation}
is the smallest nonzero combination frequency formed by the layer carriers $\{\Omega_\ell\}$ at active depth~$\delta$.  For the square-root-of-prime scheme $\Omega_\ell=\sqrt{p_\ell}\,\omega_\mathrm{ref}$, the dominant contribution to $\omega^*_\delta$ comes from the nearest-neighbour beat $|\sqrt{p_{\ell+1}}-\sqrt{p_\ell}|$, which decreases as $\approx1/(2\sqrt{p_\delta})$ for large $\delta$ (by the prime-gap estimate).  Consequently, deep circuits require proportionally larger averaging times.

In practice the averaging window spans $N_\mathrm{per}$ carrier periods of $\omega_\mathrm{ref}$, setting the measurement time
\begin{equation}
    T_\mathrm{meas} = \frac{2\pi\,N_\mathrm{per}}{\omega_\mathrm{ref}}.
    \label{eq:Tmeas}
\end{equation}
Substituting into the error bound gives the infidelity estimate
\begin{equation}
    1-\mathcal{F} \lesssim
    \frac{C_\delta\,\omega_\mathrm{ref}}{N_\mathrm{per}\,\omega^*_\delta},
    \label{eq:infidelity_bound}
\end{equation}
where $C_\delta$ is a circuit-depth-dependent constant that grows with the density of near-resonant frequency combinations at depth~$\delta$.

\subsection{Numerical convergence curves}

Figure~\ref{fig:sim_convergence} shows the infidelity $1-\mathcal{F}(N_\mathrm{per})$ on a semilogarithmic scale for three benchmark circuits of increasing depth: Bell state ($\delta=1$, 2~qubits), Grover-2 search ($\delta=2$, 2~qubits), and QFT-3 on $|001\rangle$ ($\delta=4$, 3~qubits).  All three reach $\mathcal{F}>0.999$ well within $N_\mathrm{per}=200$.  The slopes confirm the $\mathcal{O}(1/N_\mathrm{per})$ convergence of Eq.~\eqref{eq:infidelity_bound}. The Bell state converges fastest ($\omega^*_1=\sqrt{3}-\sqrt{2}\approx0.318\,\omega_\mathrm{ref}$), while QFT-3 requires more periods because the four layer frequencies at $\delta=4$ create denser near-resonant combinations.

\begin{figure}[h]
\centering
\includegraphics[width=0.7\columnwidth]{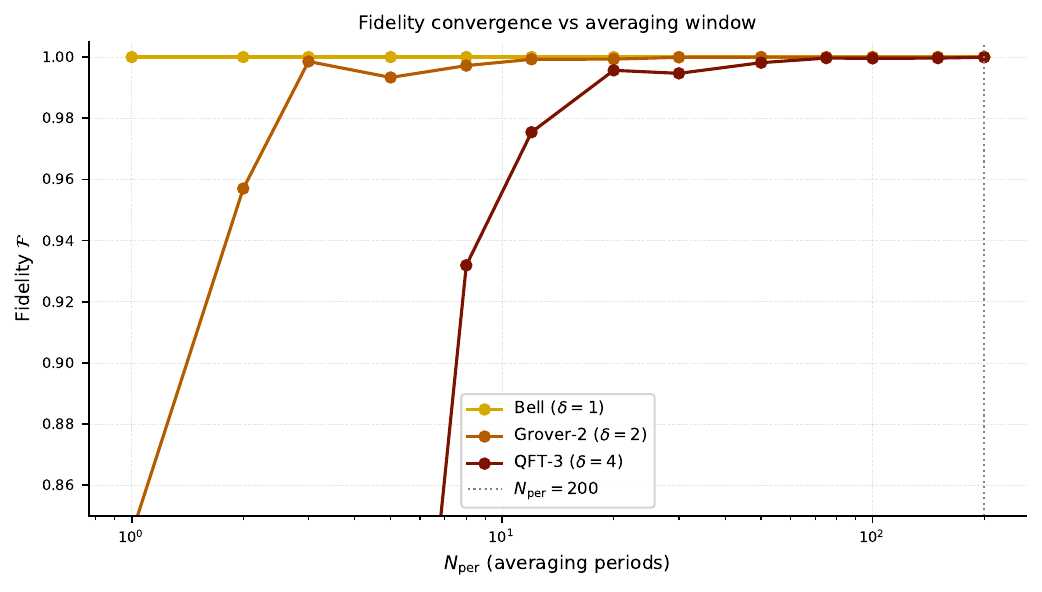}
\caption{\textbf{Fidelity convergence vs.\ averaging periods $N_\mathrm{per}$.} Semilogarithmic plot of $1-\mathcal{F}$ (infidelity) between the exact Qiskit statevector and the time-averaged wavebit simulation as a function of $N_\mathrm{per}$. Bell state ($\delta=1$, blue circles), Grover-2 ($\delta=2$, orange squares), and QFT-3 on $|001\rangle$ ($\delta=4$, green triangles). The dashed line shows the $1/N_\mathrm{per}$ slope predicted by Theorem~2. All circuits exceed $\mathcal{F}=0.999$ by $N_\mathrm{per}=200$.}
\label{fig:sim_convergence}
\end{figure}

\newpage
% ============================================================
\section{Digital Simulation: Frequency Assignment}
\label{sup:sec:S8_freqassign}
% ============================================================

\subsection{Nyquist sampling criterion}

The digital simulation evaluates $\avgT{\hat{G}(t)}$ by numerically integrating the product of $\delta$ layer matrices over $N_\mathrm{samp}$ uniformly spaced time points.  Each layer matrix $\hat{S}_\ell(t)$ oscillates at carrier frequencies $\{m\Omega_\ell\}_{m=1}^{16}$; the instantaneous product therefore contains frequencies up to
\begin{equation}
    \Omega_\mathrm{max} = \sum_{\ell=1}^{\delta}
    \max_m|m\Omega_\ell|.
    \label{eq:omegamax}
\end{equation}
By the Nyquist theorem, artifact-free integration requires $N_\mathrm{samp}\geq 2\,\Omega_\mathrm{max}\,T_\mathrm{meas}/(2\pi)$. With $T_\mathrm{meas}=2\pi N_\mathrm{per}/\omega_\mathrm{ref}$ and a conservative safety factor~16, the adaptive sampling rule used in the digital simulation is
\begin{equation}
    N_\mathrm{samp} \geq 32\,N_\mathrm{per}
    \sqrt{\frac{p_{\delta}}{2}},
    \label{eq:N_nyquist}
\end{equation}
where $p_{\delta}$ is the $\delta$-th prime and the factor~$1/2$ accounts for the half-integer frequency-index structure of the layer carrier assignment.

\subsection{Comparison of frequency schemes}

Table~\ref{tab:freq_comparison} compares three candidate carrier frequency assignments in terms of $\mathbb{Q}$-independence and the resulting $N_\mathrm{samp}$ scaling.

\begin{table}[h]
\centering
\caption{Carrier frequency scheme comparison for a depth-$\delta$ circuit. $\mathbb{Q}$-ind.\ = linearly independent over~$\mathbb{Q}$.}
\label{tab:freq_comparison}
\begin{ruledtabular}
\begin{tabular}{lccc}
Scheme & $\mathbb{Q}$-ind. & $\Omega_\mathrm{max}$ scaling
       & $N_\mathrm{samp}$ scaling \\
\hline
Harmonic, $\ell\,\omega_\mathrm{ref}$ & No & $\delta\,\omega_\mathrm{ref}$ & ill-defined \\
Power-of-$\pi$, $\pi^\ell\omega_\mathrm{ref}$ & Yes & $\pi^\delta\,\omega_\mathrm{ref}$ & $\mathcal{O}(e^{\delta\ln\pi/2})$ \\
$\sqrt{\text{prime}}$, $\sqrt{p_\ell}\,\omega_\mathrm{ref}$ & Yes
  & $\sqrt{p_\delta}\,\omega_\mathrm{ref}$ & $\mathcal{O}(\delta^{1/2}\ln^{1/2}\delta)$ \\
\end{tabular}
\end{ruledtabular}
\end{table}

\textit{Harmonic scheme.}  Setting $\Omega_\ell=\ell\,\omega_\mathrm{ref}$
produces rational ratios and therefore $\mathbb{Q}$-linear dependence (Lemma~\ref{lem:rational}, Appendix~\ref{app:thm1} of the main text).  Combination frequencies can sum to zero for nontrivial $\mathbf{k}\neq\mathbf{0}$, causing the time-averaged product to include spurious non-zero cross-terms; the averaging identity of Theorem~1 does not hold.

\textit{Power-of-$\pi$ scheme.}  Choosing $\Omega_\ell=\pi^\ell\,\omega_\mathrm{ref}$
gives $\mathbb{Q}$-independence because $\{\pi,\pi^2,\ldots\}$ are transcendentally independent.  However, $\Omega_\mathrm{max}$ grows as $\pi^\delta$, making $N_\mathrm{samp}\propto N_\mathrm{per}\cdot\pi^{\delta/2}$ exponential in circuit depth and impractical beyond $\delta\approx10$.

\textit{$\sqrt{\text{prime}}$ scheme.}  The assignment
$\Omega_\ell=\sqrt{p_\ell}\,\omega_\mathrm{ref}$ achieves $\mathbb{Q}$-independence via Besicovitch's theorem and keeps $\Omega_\mathrm{max}\propto\sqrt{p_\delta}$. By the prime number theorem $p_\delta\sim\delta\ln\delta$, so $N_\mathrm{samp}$ grows as $(\delta\ln\delta)^{1/2}$ — sub-linear in depth, allowing circuits with $\delta\sim10^2$ to be simulated on commodity hardware.  All digital simulations in this work use this scheme with $\omega_\mathrm{ref}$ absorbed into the time unit ($\Omega_\ell=\sqrt{p_\ell}$).

\newpage
% ============================================================
\section{Digital Simulation: Code Structure and Extended Results}
\label{sup:sec:S10_simresults}
% ============================================================

This section describes the structure of the digital simulation (\texttt{wavebit\_testbench.ipynb}) and presents extended diagnostic figures for all six benchmark circuits.

\subsection{Code architecture}
\label{subsec:S10_code}

The simulation is built around a \texttt{WaveBitTestBench} class that wraps a Qiskit \texttt{QuantumCircuit} and replicates it in the wavebit formalism.  The main execution pipeline is:

\begin{enumerate}
  \item \textbf{Gate decomposition.}
    \texttt{unravel\_2qubit\_gate(U)} decomposes each $4\times4$ gate into
    two $2\times2$ layer matrices $\hat{S}_1(t)$ and $\hat{S}_2(t)$
    following the construction of Appendix~\ref{app:gate_expand} of the main text.

  \item \textbf{Frequency assignment.}
    \texttt{layer\_frequency(layer\_idx, element\_idx)} assigns carrier
    frequencies $\Omega_\ell = \sqrt{p_\ell}\,\omega_\mathrm{ref}$ using the
    square-root-of-prime scheme (Sec.~\ref{sup:sec:S8_freqassign}), with a
    distinct prime for each layer–element pair to guarantee
    $\mathbb{Q}$-linear independence.

  \item \textbf{Adaptive sampling.}
    \texttt{adaptive\_n\_samples(n\_per, circuit\_depth)} applies
    Eq.~\eqref{eq:N_nyquist} to determine $N_\mathrm{samp}$: the
    minimum sample count needed to resolve the highest frequency in the
    product signal without aliasing.

  \item \textbf{Time averaging.}
    \texttt{time\_average(signal, t\_grid)} numerically integrates the
    instantaneous tensor-product signal
    $|\psi_1(t)\rangle\otimes|\psi_2(t)\rangle\otimes\cdots$
    over a uniform grid of $N_\mathrm{samp}$ points spanning
    $T_\mathrm{meas}=2\pi N_\mathrm{per}/\omega_\mathrm{ref}$.

  \item \textbf{Fidelity evaluation.}
    The time-averaged state is compared against the exact Qiskit
    statevector via $\mathcal{F}=|\langle\psi_q|\Psi_w\rangle|^2$
    (amplitude-weighted, global-phase-corrected).
\end{enumerate}

Six benchmark circuits are pre-defined: Bell state, Grover-2 ($k=1$ iteration), three-qubit W$_3$ state, QFT-3 on $|001\rangle$, Deutsch-Jozsa-4 (balanced oracle), and Deutsch-Jozsa-4 (constant oracle, $\delta=0$).  A custom circuit slot accepts arbitrary Qiskit circuits.

\subsection{Time-domain waveform evolution through the Bell circuit}
\label{subsec:S10_traces}

Figure~\ref{fig:supp_time_traces} shows the time-domain waveforms of all four dynamic amplitudes $\alpha_0^{(1)}(t)$, $\alpha_1^{(1)}(t)$, $\alpha_0^{(2)}(t)$, $\alpha_1^{(2)}(t)$ at three stages of the Bell State Generation Circuit, tracing the signal evolution from input to output.

\begin{figure*}[htbp]
\centering
\includegraphics[width=\textwidth]{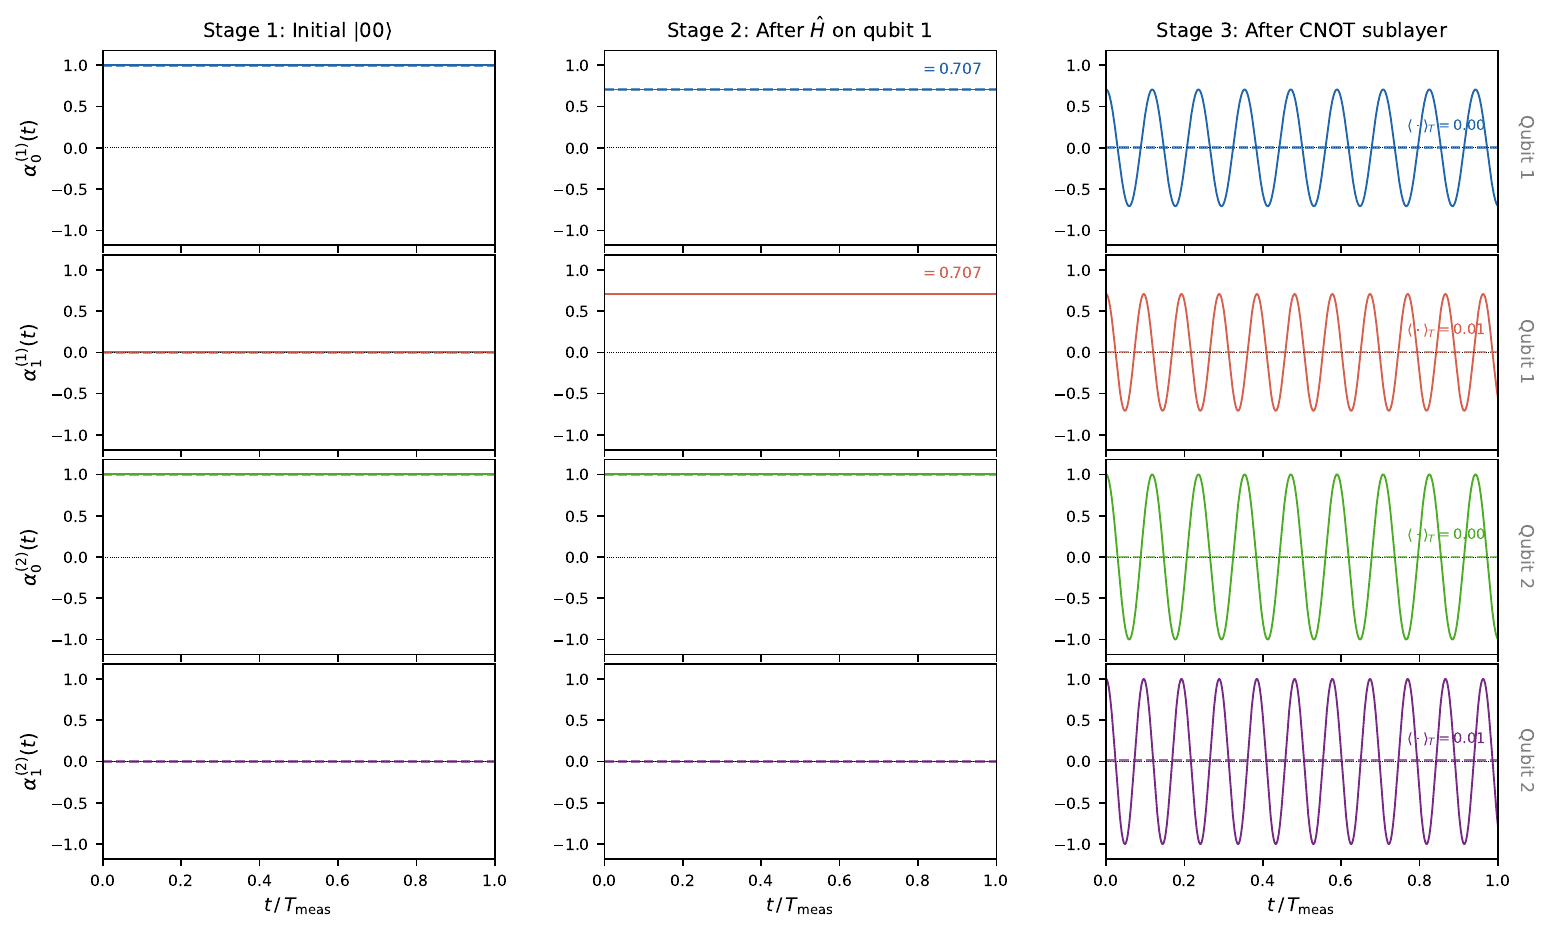}
\caption{\textbf{Coefficient waveforms through the Bell circuit.} All four dynamic amplitudes vs.\ normalised time $t/T_\mathrm{meas}$ at three stages: \textit{left}: initial state $|00\rangle$ before the Hadamard (all coefficients constant); \textit{centre}: after $\hat{H}$ applied to qubit~1 via the static matrix $\hat{C}_1$ (qubit~1 amplitudes become time-varying; qubit~2 unchanged); \textit{right}: after the CNOT layer $\hat{S}_1(t)\otimes\hat{S}_2(t)$ (both wavebits oscillate at mixed frequencies). The time average of the right-panel product $\alpha_0^{(1)}\alpha_0^{(2)}$ recovers $1/\sqrt{2}$; $\alpha_1^{(1)}\alpha_1^{(2)}$ recovers $1/\sqrt{2}$; all other products average to zero — giving $|\Phi^+\rangle$.}
\label{fig:supp_time_traces}
\end{figure*}

\subsection{Density matrices}
\label{subsec:S10_density}

Figure~\ref{fig:supp_density} shows the absolute value $|\rho_{ij}|$ of the density matrix $\rho=|\Psi\rangle\langle\Psi|$ for each circuit. Both on-diagonal (probability) and off-diagonal (coherence) elements agree between the exact Qiskit statevector and the time-averaged wavebit simulation, confirming full density-matrix reproduction.

\begin{figure*}[htbp]
\centering
\includegraphics[width=\textwidth]{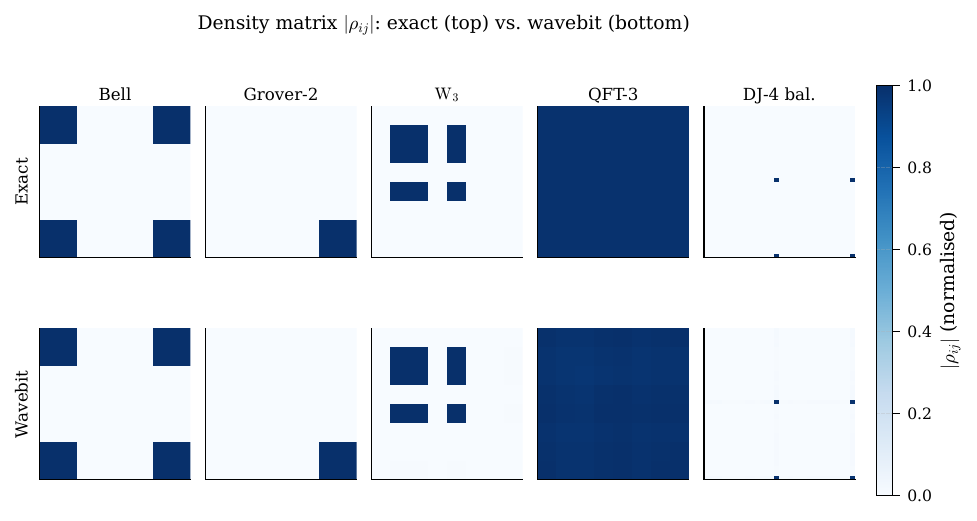}
\caption{\textbf{Density matrix $|\rho_{ij}|$ for all six benchmark circuits.} Columns: Bell, Grover-2, W$_3$, QFT-3, DJ-4 balanced, DJ-4 constant. Top row: exact Qiskit statevector. Bottom row: wavebit simulation ($N_\mathrm{per}=200$, $\sqrt{\mathrm{prime}}$ scheme). Color encodes $|\rho_{ij}|$ normalised to the maximum across both rows for each circuit. Both on-diagonal (probabilities) and off-diagonal (coherences) elements agree to within the simulation error.}
\label{fig:supp_density}
\end{figure*}

\subsection{Amplitude and phase decomposition}
\label{subsec:S10_amp}

Figure~\ref{fig:supp_amp_phase} decomposes the output statevector into amplitude $|\alpha_\mathbf{b}|$ and complex phase $\arg(\alpha_\mathbf{b})$ for each computational-basis state.

\begin{figure*}[htbp]
\centering
\includegraphics[width=\textwidth]{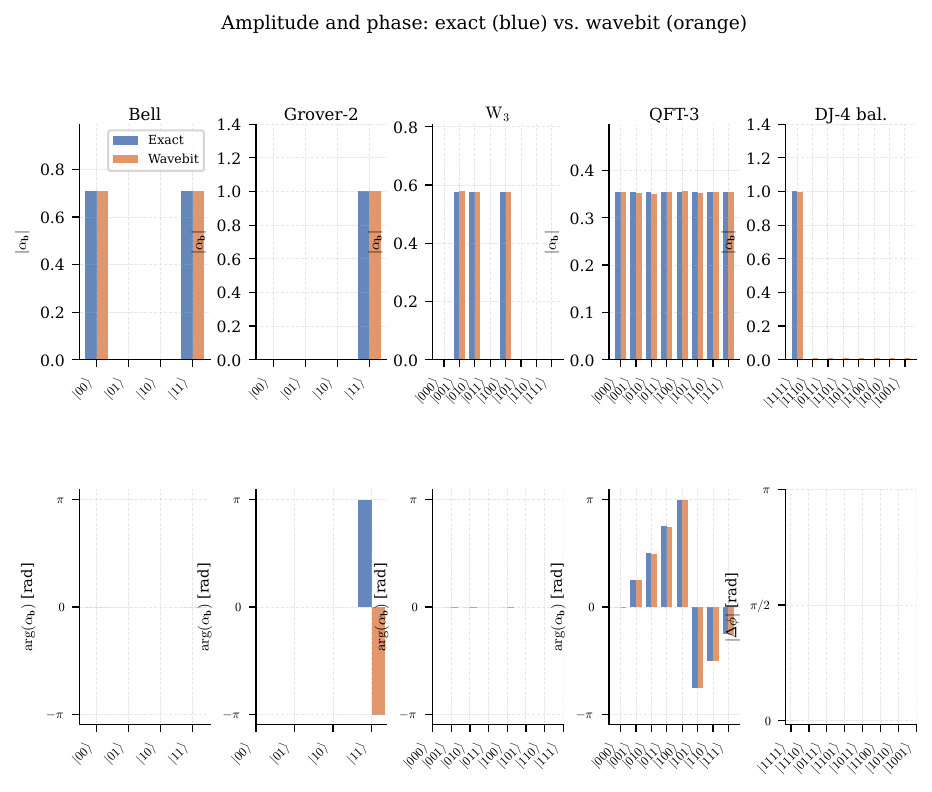}
\caption{\textbf{Amplitude and phase decomposition for all six benchmark circuits.} Each column corresponds to one circuit. \textit{Top:} Statevector amplitude $|\alpha_\mathbf{b}|$ for exact Qiskit (blue) and wavebit (orange). \textit{Bottom:} Complex phase $\arg(\alpha_\mathbf{b})$ (in radians) for states with $|\alpha_\mathbf{b}|>10^{-3}$; for the DJ-4 balanced circuit (input-register marginal), the absolute phase difference $|\Delta\phi|$ is shown instead. All circuits at $N_\mathrm{per}=200$, $\sqrt{\mathrm{prime}}$ scheme.}
\label{fig:supp_amp_phase}
\end{figure*}

\begin{comment}
Figure~\ref{fig:supp_probs} provides a probability comparison for all five circuits.

\begin{figure*}[htbp]
\centering
\includegraphics[width=\textwidth]{figures/fig_supp_probs_panel.pdf}
\caption{\textbf{Output probabilities (all five circuits).} Top-8 basis-state probabilities for exact Qiskit (blue) and wavebit (orange); $N_\mathrm{per}=200$, $\sqrt{\text{prime}}$ scheme. Fidelity $\mathcal{F}$ is quoted in each panel title.}
\label{fig:supp_probs}
\end{figure*}
\end{comment}
\bibliographystyle{apsrev4-2}
\bibliography{refs_merged}

\end{document}
